# Supplementary material for: Learning Answer Generation using Supervision from Automatic Question Answering Evaluators
Source: arXiv:2305.15344 source file (2023-05-24)
Supplement: Supplementary file 1 [file appendix.tex]

\section*{Appendix}

\section{Implementation details}
\label{apx:implementationdetails}
